# Supplementary material for: Joint Modelling of Quantum and Classical Noise over Unity Quantum Channel
Source: arXiv:2206.03894 source file (2022-06-08)
Supplement: Supplementary file 1 [file appendix-old.tex]

\vspace{-0.7 cm}
 \textcolor{blue}{\appendix[Mathematical explanation of approximating the qubit by a single variable function:]}
 \textcolor{blue}{\textit{ Representation of a qubit :}}
      \textcolor{blue}{Case I: \textit{A qubit can be represented by a point $(\theta,\phi)$ on the Bloch sphere:} A qubit on the Bloch sphere can be viewed as a pure state qubit, and it can be represented by a bivariate function $\zeta (\theta,\phi)$, it is clear from the notation that $\zeta$ is bivariate function, whose arguments are $\theta$ and $\phi$, which we call variables $x_1$ and $x_2$ respectively.} 
    \textcolor{blue}{ Case II: \textit{A qubit can be represented by a point $(\theta,\phi,r)$ inside the Bloch sphere :} A qubit inside the Bloch sphere can be viewed as a mixed state qubit, and it can be represented by a multivariate function $\tilde{\zeta} (\theta,\phi,r)$, whose arguments are $\theta$, $\phi$ and $r$, which we call variables $x_1$, $x_2$ and $x_3$ respectively.}
          
    \textcolor{blue}{\textit{ Assumption related to joint quantum noise effects:} In classical communication theory and control theory, it is found that there is a high probability that the bits will remain within a certain region of the actual position due a certain range of noise power, which is practically observed. Though it can happen that the bit may travel beyond this region, in that case the noise power would be extremely high, which is not usually observed in practice. The quantum noise can be usually observed when the classical noise has been suppressed. Since we are considering the classical noise along with the quantum noise, and  so when we considering both at a time it is a obvious choice to consider the above noise power theory as already the classical noise is integrated in the system and it effects should be reflected on the calculations. In connection to  control theory, we can infer that within a certain (practical) range of the joint noise power, the qubit will not move far beyond from its actual position due to the joint noise effect. This works for both the pure state and the mixed state qubits.\\}
    \textcolor{blue}{Case I: \textit{ We now consider the pure state qubit, and we will discuss how its position is affected by the noise power:} \\
    In Fig.~\ref{fig Bloch sphere representation_2}, the qubit is lying on the surface of the Bloch sphere. In this case the pure state qubit can be represented as a  bivariate function of $(\theta, \phi)$. We assume that within a certain noise power the qubit will remain within a complete strip along the surface of the Bloch sphere. In particular we consider a circular path along the surface of the sphere, which will be the path of the qubit if one rotates the qubit by varying $\theta$ while keeping $\phi$ constant. Now consider a strip along the surface of the sphere that contains the path circle of the qubit in the middle, then the distance from the qubit on the circle to the edges of the strip will be $\delta$ on each side, hence the  breath of the strip will be $2\delta$. We consider that if the qubit will experience a certain (practically feasible) range of the noise power, then the position of the qubit will not end up far beyond the indicated region (the strip). 
    Mathematically, we considered $(\theta , \phi) \mapsto (\tilde{\theta} , \phi \pm \delta)$ where $\tilde{\theta} \in [0, 2\pi]$. 
    And to reduce the computational complexity of the problem, we infer that the $\delta$ will be so small that the second variable $\phi$ can be thought of as constant with respect to $\theta$.}
          \vspace{-0.7 cm}
          
         \begin{figure}[htbp]
          \centering
          \subfloat[]{
          \includegraphics[width=0.47\columnwidth]{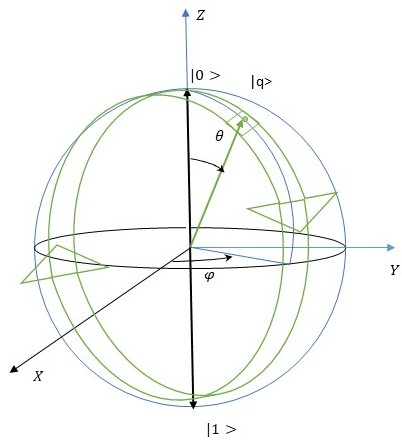}
          \label{fig Case I  }
          }
         \hfill
         \subfloat[]{
         %\centering
         \includegraphics[width=0.47\columnwidth]{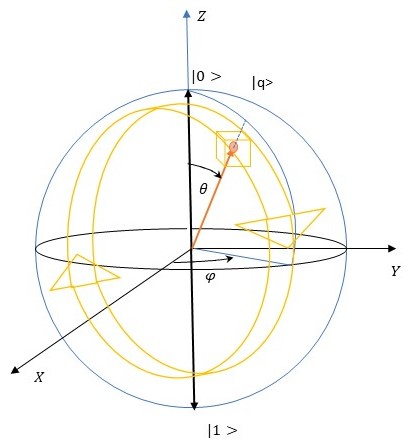}
         \label{fig Case II}
         %\end{subfigure}
         }
        \hfill
         \caption{(a) Case I: when the qubit is on the Bloch sphere, and (b) Case II: when the qubit is inside the Bloch sphere.}
         \label{fig Bloch sphere representation_2}
         \end{figure}
         
\textcolor{blue}{ Case II: \textit{ We are considering the mixed state qubit, and we will discuss its position affected by the noise power:} \\
 When we are dealing with the qubit that is lying inside the Bloch sphere, the pure state qubit can be represented as a multivariate function of $(\theta, \phi,r)$, where $r$ is the distance of the qubit from the center of the sphere. In connection to control theory, we infer that within a certain (feasible) range of noise power the qubit will remain within a torus/tunnel-like object (whose cross section is square) inside the Bloch sphere. Consider a  circular path inside the sphere which will be the path of the qubit, if one rotates the qubit by varying $\theta$ while keeping $\phi$ and $r$ constant. Now consider a torus/tunnel-like object (whose cross section is square) inside the sphere that contains the path circle of the qubit in the middle, the distance from the qubit on the circle to the sides of the tunnel will be $\delta$ in each of sides of cube, hence the area of the cross-sectional region (which is a square) will be $2\delta$ x $ 2\delta$. We consider that if the qubit will experience a certain (practically feasible) range for the noise power, then the position of the qubit will not go far beyond the indicated region (the torus /tunnel). }
 
\textcolor{blue}{Mathematically, we considered $(\theta , \phi, r) \mapsto (\tilde{\theta} , \phi \pm \delta_{1}, r \pm \delta_{2})$ where $\tilde{\theta} \in [0, 2\pi]$. For reducing the complexity,we can infer that that cuboid region can be approximated by the cube region that we discussed above. Hence we have, 
 $(\theta , \phi, r) \mapsto (\tilde{\theta} , \phi \pm \delta, r \pm \delta)$ where $\tilde{\theta} \in [0, 2\pi]$.Now we expect that the $\delta$ will be so small that the second and third variables $\phi$ and $r$ can be thought of as constant with respect to first variable $\theta$. Therefore we have, $(\theta , \phi, r) \mapsto (\tilde{\theta} , \phi , r )$ where $\tilde{\theta} \in [0, 2\pi]$.}
         
         
         
         %\begin{figure}[htbp]
         %\centerline{\includegraphics[width = 0.95\columnwidth]{}}
         %\caption{\label{fig Characterization of joint noise}
         %\end{figure}
\textcolor{blue}{In summary, this approximation can be done by varying any one of the variables $\theta$ and $\phi$ at a time, considering the other variables as constant with respect to said variable. In our case we varied $\theta$, considering the rest of the variables as constant.   
}
